# Supplementary material for: Reference Vertical Excitation Energies for Transition Metal Compounds
Source: arXiv:2309.17311 ancillary file (2023-11-14)
Supplement: Supplementary file 1 [file TM_SI.pdf]

# Supporting Information for "Reference Vertical Excitation Energies for Transition Metal Compounds"

Denis Jacquemin,[1, 2, a)] Fábris Kossoski,[3] Franck Gam,[1] Martial Boggio-Pasqua,[3, b)] and Pierre-François Loos[3, c)]
[1)] *Nantes Université, CNRS, CEISAM UMR 6230, F-44000 Nantes, France*
[2)] *Institut Universitaire de France (IUF), F-75005 Paris, France*
[3)] *Laboratoire de Chimie et Physique Quantiques (UMR 5626), Université de Toulouse, CNRS, UPS, France*

In the following tables, we report the vertical transition energies (in eV) obtained with the aug-cc-pVTZ and aug-cc-pVDZ basis sets and computed with state-averaged CASSCF, state-specific CASPT2 and NEVPT2. Whenever possible, the CASPT2 calculations were performed with the RS2 contraction scheme, but for a few cases the more contracted version RS2C had to be used (denoted CASPT2C in the tables). A level shift of 0.30 $E_h$ was systematically used. The CASPT2 calculations were performed with (IPEA) and without (NOIPEA) the IPEA shift. The standard value of 0.25 $E_h$ was used when the IPEA correction is included. Also, in a few cases, the density-fitting approximation on the 2-electron integrals was used (as indicated in some table footnotes). The NEVPT2 calculations were performed in both the partially-contracted (PC-) and strongly-contracted (SC-) versions. Canonical orbitals were generated for each state in these calculations. All calculations are reported using a large core, as used in the CC calculations but for some cases the effect of using a smaller core is reported. The composition of the active space is specified in terms of number of active orbitals per irreducible representation. The state-averaging procedure used is also described in terms of number of states per irreducible representation. Note that, for all calculations, the ground state is systematically included in the state-averaging procedure even if it does not belong to the same irreducible representation. The Cartesian coordinates have been extracted from the QUEST database (M. Véril, A. Scemama, M. Caffarel, F. Lipparini, M. Boggio-Pasqua, D. Jacquemin, and P.-F. Loos, WIREs Comput. Mol. Sci. **11**, e1517 (2021)) and can be downloaded at https://lcpq.github.io/QUESTDB_website.

[a)] Electronic mail: denis.jacquemin@univ-nantes.fr
[b)] Electronic mail: martial.boggio@irsamc.ups-tlse.fr
[c)] Electronic mail: loos@irsamc.ups-tlse.fr

## A. ScH and ScF

**Table S1.** Vertical transition energies (eV) of ScH with aug-cc-pVTZ basis set.

| State | Active space ($a_1,b_1,b_2,a_2$) | State-average ($A_1,B_1,B_2,A_2$) | CASSCF[a] | CASPT2 NOIPEA (9 core)[b] | CASPT2 IPEA (9 core)[b] | CASPT2 NOIPEA (5 core)[c] | CASPT2 IPEA (5 core)[c] | SC-NEVPT2 (9 core)[b] | PC-NEVPT2 (9 core)[b] | SC-NEVPT2 (5 core)[c] | PC-NEVPT2 (5 core)[c] |
|---|---|---|---|---|---|---|---|---|---|---|---|
| $^1\Delta$ | (5,2,2,1) | (2,0,0,1) | 0.490 | **0.514** | **0.515** | **0.562** | **0.582** | **0.532** | **0.535** | **0.590** | **0.596** |
| $^1\Pi$ | (5,2,2,1) | (1,1,1,0) | 0.814 | **0.742** | **0.764** | **0.740** | **0.794** | **0.774** | **0.769** | **0.772** | **0.769** |
| $^1\Sigma^+$ | (5,2,2,1) | (2,0,0,0) | 2.310 | **1.920** | **2.040** | **1.683** | **1.868** | **2.003** | **1.983** | **1.766** | **1.744** |
| $^1\Pi$ | (5,2,2,1) | (1,2,2,0) | 2.115 | **2.077** | **2.129** | **2.040** | **2.149** | **2.153** | **2.149** | **2.202** | **2.199** |
| $^3\Delta$ | (5,2,2,1) | (2,0,0,1) | 0.270 | **0.278** | **0.280** | **0.271** | **0.294** | **0.293** | **0.295** | **0.301** | **0.306** |
| $^3\Pi$ | (5,2,2,1) | (1,1,1,0) | 0.537 | **0.496** | **0.510** | **0.483** | **0.528** | **0.523** | **0.523** | **0.510** | **0.511** |
| $^3\Sigma^+$ | (5,2,2,1) | (2,0,0,0) | 0.833 | **0.785** | **0.813** | **0.804** | **0.865** | **0.825** | **0.827** | **0.887** | **0.890** |
| $^3\Pi$ | (5,2,2,1) | (1,2,2,0) | 1.812 | **1.809** | **1.853** | **1.878** | **1.950** | **1.842** | **1.839** | **1.966** | **1.964** |

[a] All calculations using a (4e,10o) active space including 4s, 3d, 4p of Sc and 1s of H.
[b] Core orbitals not correlated at PT2 level: 1s, 2s, 2p, 3s, 3p of Sc (5,2,2,0).
[c] Core orbitals not correlated at PT2 level: 1s, 2s, 2p of Sc (3,1,1,0).

**Table S2.** Vertical transition energies (eV) of ScH with aug-cc-pVDZ basis set.

| State | Active space ($a_1,b_1,b_2,a_2$) | State-average ($A_1,B_1,B_2,A_2$) | CASSCF[a] | CASPT2 NOIPEA (9 core)[b] | CASPT2 IPEA (9 core)[b] | SC-NEVPT2 (9 core)[b] | PC-NEVPT2 (9 core)[b] |
|---|---|---|---|---|---|---|---|
| $^1\Delta$ | (5,2,2,1) | (2,0,0,1) | 0.486 | **0.519** | **0.519** | **0.535** | **0.538** |
| $^1\Pi$ | (5,2,2,1) | (1,1,1,0) | 0.818 | **0.763** | **0.783** | **0.791** | **0.786** |
| $^1\Sigma^+$ | (5,2,2,1) | (2,0,0,0) | 2.308 | **1.942** | **2.060** | **2.024** | **2.003** |
| $^1\Pi$ | (5,2,2,1) | (1,2,2,0) | 2.111 | **2.071** | **2.122** | **2.146** | **2.141** |
| $^3\Delta$ | (5,2,2,1) | (2,0,0,1) | 0.267 | **0.275** | **0.278** | **0.290** | **0.292** |
| $^3\Pi$ | (5,2,2,1) | (1,1,1,0) | 0.538 | **0.507** | **0.520** | **0.533** | **0.532** |
| $^3\Sigma^+$ | (5,2,2,1) | (2,0,0,0) | 0.834 | **0.794** | **0.821** | **0.833** | **0.834** |
| $^3\Pi$ | (5,2,2,1) | (1,2,2,0) | 1.810 | **1.804** | **1.845** | **1.836** | **1.832** |

[a] All calculations using a (4e,10o) active space including 4s, 3d, 4p of Sc and 1s of H.
[b] Core orbitals not correlated at PT2 level: 1s, 2s, 2p, 3s, 3p of Sc (5,2,2,0).

**Table S3.** Vertical transition energies (eV) of ScF with aug-cc-pVTZ basis set.

| State | Active space ($a_1,b_1,b_2,a_2$) | State-average ($A_1,B_1,B_2,A_2$) | CASSCF[a] | CASPT2 NOIPEA (10 core)[b] | CASPT2 IPEA (10 core)[b] | CASPT2 NOIPEA (6 core)[c] | CASPT2 IPEA (6 core)[c] | SC-NEVPT2 (10 core)[b] | PC-NEVPT2 (10 core)[b] | SC-NEVPT2 (6 core)[c] | PC-NEVPT2 (6 core)[c] |
|---|---|---|---|---|---|---|---|---|---|---|---|
| $^1\Delta$ | (5,2,2,1) | (2,0,0,1) | 0.506 | **0.550** | **0.554** | **0.598** | **0.631** | **0.568** | **0.584** | **0.569** | **0.594** |
| $^1\Pi$ | (5,2,2,1) | (1,1,1,0) | 1.265 | **1.318** | **1.344** | **1.330** | **1.404** | **1.394** | **1.409** | **1.307** | **1.322** |
| $^1\Sigma^+$ | (5,2,2,1) | (2,0,0,0) | 2.490 | **2.278** | **2.366** | **2.004** | **2.169** | **2.390** | **2.382** | **2.071** | **2.055** |
| $^1\Pi$ | (5,2,2,1) | (1,2,2,0) | 2.337 | **2.421** | **2.478** | **2.468** | **2.591** | **2.560** | **2.569** | **2.638** | **2.650** |
| $^3\Delta$ | (5,2,2,1) | (2,0,0,1) | 0.262 | **0.288** | **0.292** | **0.279** | **0.313** | **0.312** | **0.318** | **0.257** | **0.267** |
| $^3\Pi$ | (5,2,2,1) | (1,1,1,0) | 0.840 | **0.885** | **0.896** | **0.860** | **0.908** | **0.928** | **0.933** | **0.816** | **0.819** |
| $^3\Sigma^+$ | (5,2,2,1) | (2,0,0,0) | 1.391 | **1.366** | **1.389** | **1.302** | **1.362** | **1.396** | **1.408** | **1.311** | **1.323** |
| $^3\Pi$ | (5,2,2,1) | (1,2,2,0) | 2.263 | **2.393** | **2.422** | **2.427** | **2.516** | **2.496** | **2.503** | **2.504** | **2.513** |

[a] Using a reference (4e,10o) active space including 4s, 3d, 4p of Sc and $2p_z$ of F.

[b] Core orbitals not correlated at PT2 level: 1s, 2s, 2p, 3s, 3p of Sc and 1s of F (6,2,2,0).

[c] Core orbitals not correlated at PT2 level: 1s, 2s, 2p of Sc and 1s of F (4,1,1,0).

**Table S4.** Vertical transition energies (eV) of ScF with aug-cc-pVDZ basis set.

| State | Active space ($a_1,b_1,b_2,a_2$) | State-average ($A_1,B_1,B_2,A_2$) | CASSCF[a] | CASPT2 NOIPEA (10 core)[b] | CASPT2 IPEA (10 core)[b] | SC-NEVPT2 (10 core)[b] | PC-NEVPT2 (10 core)[b] |
|---|---|---|---|---|---|---|---|
| $^1\Delta$ | (5,2,2,1) | (2,0,0,1) | 0.494 | **0.556** | **0.559** | **0.597** | **0.612** |
| $^1\Pi$ | (5,2,2,1) | (1,1,1,0) | 1.243 | **1.330** | **1.353** | **1.391** | **1.406** |
| $^1\Sigma^+$ | (5,2,2,1) | (2,0,0,0) | 2.471 | **2.292** | **2.378** | **2.391** | **2.385** |
| $^1\Pi$ | (5,2,2,1) | (1,2,2,0) | 2.323 | **2.427** | **2.479** | **2.553** | **2.562** |
| $^3\Delta$ | (5,2,2,1) | (2,0,0,1) | 0.251 | **0.288** | **0.292** | **0.336** | **0.341** |
| $^3\Pi$ | (5,2,2,1) | (1,1,1,0) | 0.820 | **0.885** | **0.896** | **0.919** | **0.923** |
| $^3\Sigma^+$ | (5,2,2,1) | (2,0,0,0) | 1.370 | **1.367** | **1.389** | **1.392** | **1.403** |
| $^3\Pi$ | (5,2,2,1) | (1,2,2,0) | 2.244 | **2.382** | **2.409** | **2.472** | **2.478** |

[a] Using a reference (4e,10o) active space including 4s, 3d, 4p of Sc and $2p_z$ of F.

[b] Core orbitals not correlated at PT2 level: 1s, 2s, 2p, 3s, 3p of Sc and 1s of F (6,2,2,0).

## B. CuH, CuF and CuCl

**Table S5.** Vertical transition energies (eV) of CuH with aug-cc-pVTZ basis set.

| State | Active space ($a_1,b_1,b_2,a_2$) | State-average ($A_1,B_1,B_2,A_2$) | CASSCF[a] | CASPT2 NOIPEA (9 core)[b] | CASPT2 IPEA (9 core)[b] | CASPT2C NOIPEA (5 core)[c] | CASPT2C IPEA (5 core)[c] |
|---|---|---|---|---|---|---|---|
| $^1\Sigma^+(d_{z^2},4s)$ | (7,3,3,2) | (2,0,0,0) | 2.642 | **3.067** | **3.143** | **2.976** | **3.068** |
| $^1\Pi(d_{xz}/d_{yz},4s)$ | (7,3,3,2) | (1,1,1,0) | 2.784 | **3.652** | **3.623** | **3.569** | **3.553** |
| $^1\Delta(d_{xy}/d_{x^2-y^2},4s)$ | (7,3,3,2) | (2,0,0,1) | 2.756 | **3.642** | **3.614** | **3.560** | **3.544** |
| $^1\Pi(d_{z^2}/d_{yz},4s)$ | (7,3,3,2) | (1,2,2,0) | 4.656 | **5.260** | **5.449** | **5.192** | **5.397** |
| $^1\Sigma^+(d_{z^2},4p_x/4p_y)$ | (7,3,3,2) | (3,0,0,0) | 5.516 | **5.932** | **6.038** | **5.878** | **5.995** |
| $^3\Sigma^+(d_{z^2},4s)$ | (7,3,3,2) | (2,0,0,0) | 2.082 | **2.507** | **2.572** | **2.409** | **2.491** |
| $^3\Pi(d_{xz}/d_{yz},4s)$ | (7,3,3,2) | (1,1,1,0) | 2.523 | **3.428** | **3.393** | **3.342** | **3.321** |
| $^3\Delta(d_{xy}/d_{x^2-y^2},4s)$ | (7,3,3,2) | (2,0,0,1) | 2.611 | **3.509** | **3.479** | **3.416** | **3.401** |
| $^3\Pi(d_{z^2}/d_{yz},4s)$ | (7,3,3,2) | (1,2,2,0) | 3.973 | **4.651** | **4.746** | **4.594** | **4.702** |

[a] All calculations using a (12e,15o) active space including 4s, 3d, 4p, 4d of Cu and 1s of H.
[b] Core orbitals not correlated at PT2 level: 1s, 2s, 2p, 3s, 3p of Cu (5,2,2,0).
[c] Core orbitals not correlated at PT2 level: 1s, 2s, 2p of Cu (3,1,1,0).

**Table S6.** Vertical transition energies (eV) of CuH with aug-cc-pVDZ basis set.

| State | Active space ($a_1,b_1,b_2,a_2$) | State-average ($A_1,B_1,B_2,A_2$) | CASSCF[a] | CASPT2 NOIPEA (9 core)[b] | CASPT2 IPEA (9 core)[b] |
|---|---|---|---|---|---|
| $^1\Sigma^+(d_{z^2},4s)$ | (7,3,3,2) | (2,0,0,0) | 2.652 | **3.031** | **3.102** |
| $^1\Pi(d_{xz}/d_{yz},4s)$ | (7,3,3,2) | (1,1,1,0) | 2.803 | **3.607** | **3.571** |
| $^1\Delta(d_{xy}/d_{x^2-y^2},4s)$ | (7,3,3,2) | (2,0,0,1) | 2.798 | **3.593** | **3.558** |
| $^1\Pi(d_{z^2}/d_{yz},4s)$ | (7,3,3,2) | (1,2,2,0) | 4.683 | **5.216** | **5.408** |
| $^1\Sigma^+(d_{z^2},4p_x/4p_y)$ | (7,3,3,2) | (3,0,0,0) | 5.521 | **5.864** | **5.971** |
| $^3\Sigma^+(d_{z^2},4s)$ | (7,3,3,2) | (2,0,0,0) | 2.101 | **2.471** | **2.536** |
| $^3\Pi(d_{xz}/d_{yz},4s)$ | (7,3,3,2) | (1,1,1,0) | 2.542 | **3.374** | **3.333** |
| $^3\Delta(d_{xy}/d_{x^2-y^2},4s)$ | (7,3,3,2) | (2,0,0,1) | 2.655 | **3.457** | **3.422** |
| $^3\Pi(d_{z^2}/d_{yz},4s)$ | (7,3,3,2) | (1,2,2,0) | 3.992 | **4.601** | **4.691** |

[a] All calculations using a (12e,15o) active space including 4s, 3d, 4p, 4d of Cu and 1s of H.
[b] Core orbitals not correlated at PT2 level: 1s, 2s, 2p, 3s, 3p of Cu (5,2,2,0).

**Table S7.** Vertical transition energies (eV) of CuF with aug-cc-pVTZ basis set.

| State | Active space $(a_1,b_1,b_2,a_2)$ | State-average $(A_1,B_1,B_2,A_2)$ | CASSCF[a] | CASPT2C NOIPEA (10 core)[b] | CASPT2C IPEA (10 core)[b] |
|---|---|---|---|---|---|
| $^1\Sigma^+(d_{z^2},4s)$ | (7,3,3,2) | (2,0,0,0) | 2.076 | **2.477** | **2.539** |
| $^1\Pi(d_{xz}/d_{yz},4s)$ | (7,3,3,2) | (1,1,1,0) | 2.031 | **2.658** | **2.674** |
| $^1\Delta(d_{xy}/d_{x^2-y^2},4s)$ | (7,3,3,2) | (2,0,0,1) | 2.349 | **3.045** | **3.045** |
| $^1\Pi(d_{z^2}/d_{yz},4s)$ | (7,3,3,2) | (1,2,2,0) | 5.092 | **6.021** | **6.047** |
| $^3\Sigma^+(d_{z^2},4s)$ | (7,3,3,2) | (2,0,0,0) | 1.497 | **1.933** | **1.987** |
| $^3\Pi(d_{xz}/d_{yz},4s)$ | (7,3,3,2) | (1,1,1,0) | 1.679 | **2.355** | **2.367** |
| $^3\Delta(d_{xy}/d_{x^2-y^2},4s)$ | (7,3,3,2) | (2,0,0,1) | 2.103 | **2.791** | **2.793** |
| $^3\Pi(d_{z^2}/d_{yz},4s)$ | (7,3,3,2) | (1,2,2,0) | 4.875 | **5.790** | **5.825** |

[a] All calculations using a (12e,15o) active space including 4s, 3d, 4p, 4d of Cu and $2p_z$ of F.

[b] Core orbitals not correlated at PT2 level: 1s, 2s, 2p, 3s, 3p of Cu and 1s of F (6,2,2,0).

**Table S8.** Vertical transition energies (eV) of CuF with aug-cc-pVDZ basis set.

| State | Active space $(a_1,b_1,b_2,a_2)$ | State-average $(A_1,B_1,B_2,A_2)$ | CASSCF[a] | CASPT2C NOIPEA (10 core)[b] | CASPT2C IPEA (10 core)[b] |
|---|---|---|---|---|---|
| $^1\Sigma^+(d_{z^2},4s)$ | (7,3,3,2) | (2,0,0,0) | 2.159 | **2.471** | **2.528** |
| $^1\Pi(d_{xz}/d_{yz},4s)$ | (7,3,3,2) | (1,1,1,0) | 2.053 | **2.622** | **2.632** |
| $^1\Delta(d_{xy}/d_{x^2-y^2},4s)$ | (7,3,3,2) | (2,0,0,1) | 2.400 | **3.020** | **3.014** |
| $^1\Pi(d_{z^2}/d_{yz},4s)$ | (7,3,3,2) | (1,2,2,0) | 5.180 | **6.006** | **6.028** |
| $^3\Sigma^+(d_{z^2},4s)$ | (7,3,3,2) | (2,0,0,0) | 1.524 | **1.890** | **1.941** |
| $^3\Pi(d_{xz}/d_{yz},4s)$ | (7,3,3,2) | (1,1,1,0) | 1.708 | **2.312** | **2.317** |
| $^3\Delta(d_{xy}/d_{x^2-y^2},4s)$ | (7,3,3,2) | (2,0,0,1) | 2.152 | **2.762** | **2.758** |
| $^3\Pi(d_{z^2}/d_{yz},4s)$ | (7,3,3,2) | (1,2,2,0) | 4.957 | **5.760** | **5.791** |

[a] All calculations using a (12e,15o) active space including 4s, 3d, 4p, 4d of Cu and $2p_z$ of F.

[b] Core orbitals not correlated at PT2 level: 1s, 2s, 2p, 3s, 3p of Cu and 1s of F (6,2,2,0).

**Table S9.** Vertical transition energies (eV) of CuCl with aug-cc-pVTZ basis set.

| State | Active space ($a_1$,$b_1$,$b_2$,$a_2$) | State-average ($A_1$,$B_1$,$B_2$,$A_2$) | CASSCF | CASPT2 NOIPEA (14 core)[c] | CASPT2 IPEA (14 core)[c] | SC-NEVPT2 (14 core)[c] | PC-NEVPT2 (14 core)[c] |
|---|---|---|---|---|---|---|---|
| $^1\Sigma^+$ | (6,2,2,2)[a] | (2,0,0,0) | 2.693 | **3.018** | **3.171** | – | – |
| | (7,2,2,2)[b] | (2,0,0,0) | 2.668 | **3.009** | **3.149** | **3.047** | **3.030** |
| $^1\Pi$ | (6,2,2,2)[a] | (1,1,1,0) | 2.510 | **3.140** | **3.204** | – | – |
| | (7,2,2,2)[b] | (1,1,1,0) | 2.468 | **2.972** | **3.049** | **2.968** | **3.015** |
| $^1\Delta$ | (6,2,2,2)[a] | (2,0,0,1) | 2.698 | **3.511** | **3.536** | – | – |
| | (7,2,2,2)[b] | (2,0,0,1) | 2.554 | **3.454** | **3.472** | **3.371** | **3.454** |
| $^3\Sigma^+$ | (6,2,2,2)[a] | (2,0,0,0) | 2.195 | **2.585** | **2.721** | **2.624** | **2.597** |
| | (7,2,2,2)[b] | (2,0,0,0) | 2.159 | **2.562** | **2.692** | **2.590** | **2.578** |
| $^3\Pi$ | (6,2,2,2)[a] | (1,1,1,0) | 2.188 | **2.837** | **2.895** | – | – |
| | (7,2,2,2)[b] | (1,1,1,0) | 2.162 | **2.779** | **2.845** | **2.739** | **2.818** |
| $^3\Delta$ | (6,2,2,2)[a] | (2,0,0,1) | 2.448 | **3.257** | **3.280** | – | – |
| | (7,2,2,2)[b] | (2,0,0,1) | 2.309 | **3.214** | **3.229** | **3.124** | **3.203** |

[a] Using a (12e,12o) active space including 4s, 3d, 4d of Cu and $3p_z$ of Cl.

[b] Using a (12e,13o) active space including 4s, 3d, 4d of Cu and $3p_z$, $4p_z$ of Cl.

[c] Core orbitals not correlated at PT2 level: 1s, 2s, 2p, 3s, 3p of Cu and 1s, 2s, 2p of Cl (8,3,3,0).

**Table S10.** Vertical transition energies (eV) of CuCl with aug-cc-pVDZ basis set.

| State | Active space ($a_1$,$b_1$,$b_2$,$a_2$) | State-average ($A_1$,$B_1$,$B_2$,$A_2$) | CASSCF | CASPT2 NOIPEA (14 core)[b] | CASPT2 IPEA (14 core)[b] | SC-NEVPT2 (14 core)[b] | PC-NEVPT2 (14 core)[b] |
|---|---|---|---|---|---|---|---|
| $^1\Sigma^+$ | (7,2,2,2)[a] | (2,0,0,0) | 2.677 | **3.967** | **3.088** | **3.323** | **3.333** |
| $^1\Pi$ | (7,2,2,2)[a] | (1,1,1,0) | 2.555 | **2.902** | **2.965** | **2.929** | **2.971** |
| $^1\Delta$ | (7,2,2,2)[a] | (2,0,0,1) | 2.754 | **3.525** | **3.533** | **3.435** | **3.539** |
| $^3\Sigma^+$ | (7,2,2,2)[a] | (2,0,0,0) | 2.177 | **2.513** | **2.626** | **2.539** | **2.529** |
| $^3\Pi$ | (7,2,2,2)[a] | (1,1,1,0) | 2.235 | **2.606** | **2.661** | **2.606** | **2.654** |
| $^3\Delta$ | (7,2,2,2)[a] | (2,0,0,1) | 2.500 | **3.276** | **3.281** | **3.176** | **3.277** |

[a] Using a (12e,12o) active space including 4s, 3d, 4d of Cu and $3p_z$ of Cl.

[b] Core orbitals not correlated at PT2 level: 1s, 2s, 2p, 3s, 3p of Cu and 1s, 2s, 2p of Cl (8,3,3,0).

## C. ZnO and ZnS

**Table S11.** Vertical transition energies (eV) of ZnO with aug-cc-pVTZ basis set.

| State | Active space ($a_1$,$b_1$,$b_2$,$a_2$) | State-average ($A_1$,$B_1$,$B_2$,$A_2$) | CASSCF | CASPT2 NOIPEA (10 core)[e] | CASPT2 IPEA (10 core)[e] | CASPT3 NOIPEA (10 core)[e] | CASPT3 IPEA (10 core)[e] | SC-NEVPT2 (10 core)[e] | PC-NEVPT2 (10 core)[e] |
|---|---|---|---|---|---|---|---|---|---|
| $1^1\Pi$ | (3,2,2,0)[a] | (1,1,1,0) | 0.297 | **0.502** | **0.494** | **0.545** | **0.529** | – | – |
| | (4,2,2,0)[b] | (1,1,1,0) | 0.421 | **0.530** | **0.517** | **0.543** | **0.530** | – | – |
| | (6,3,3,1)[c] | (1,1,1,0) | 0.432 | **0.543** | **0.530** | – | – | **0.519** | **0.557** |
| | (8,4,4,2)[d] | (1,1,1,0) | 0.432[d] | **0.551**[d] | – | – | – | – | – |
| $2^1\Sigma^+$ | (3,2,2,0)[a] | (2,0,0,0) | 3.810 | **3.845** | **3.932** | **3.806** | **3.841** | **3.933** | **3.869** |
| | (4,2,2,0)[b] | (2,0,0,0) | 3.636 | **3.774** | **3.854** | **3.739** | **3.772** | **3.883** | **3.817** |
| | (6,3,3,1)[c] | (2,0,0,0) | 3.597 | **3.681** | **3.763** | – | – | **3.792** | **3.718** |
| $1^1\Delta$ | (3,2,2,0)[a] | (2,0,0,1) | 4.118 | **4.315** | **4.460** | **4.446** | **4.467** | – | – |
| | (4,2,2,0)[b] | (2,0,0,1) | 4.146 | **4.149** | **4.336** | **4.349** | **4.374** | – | – |
| | (6,3,3,1)[c] | (2,0,0,1) | 4.181 | **4.192** | **4.381** | – | – | **4.399** | **4.413** |
| $1^1\Sigma^-$ | (3,2,2,0)[a] | (1,0,0,1) | 4.573 | **4.388** | **4.647** | **4.569** | **4.643** | **4.703** | **4.618** |
| | (4,2,2,0)[b] | (1,0,0,1) | 4.816 | **4.304** | **4.664** | **4.558** | **4.663** | **4.720** | **4.568** |
| | (6,3,3,1)[c] | (1,0,0,1) | 4.823 | **4.332** | **4.692** | – | – | **4.744** | **4.587** |
| $1^3\Pi$ | (3,2,2,0)[a] | (1,1,1,0) | 0.140 | **0.310** | **0.306** | **0.347** | **0.336** | – | – |
| | (4,2,2,0)[b] | (1,1,1,0) | 0.255 | **0.332** | **0.322** | **0.340** | **0.331** | – | – |
| | (6,3,3,1)[c] | (1,1,1,0) | 0.260 | **0.342** | **0.332** | – | – | **0.323** | **0.358** |
| $1^3\Sigma^+$ | (3,2,2,0)[a] | (2,0,0,0) | 1.332 | **1.606** | **1.637** | **1.606** | **1.610** | **1.621** | **1.637** |
| | (4,2,2,0)[b] | (2,0,0,0) | 1.356 | **1.512** | **1.569** | **1.542** | **1.549** | **1.562** | **1.562** |
| | (6,3,3,1)[c] | (2,0,0,0) | 1.349 | **1.514** | **1.570** | – | – | **1.554** | **1.554** |

[a] Using a reference (6e,7o) active space including 4s, 4p of Zn and 2p of O.

[b] Using a reference (8e,8o) active space including 4s, 4p of Zn and 2s, 2p of O.

[c] Using a reference (18e,13o) active space including 4s, 3d, 4p of Zn and 2s, 2p of O.

[d] Using a reference (18e,18o) active space including 4s, 3d, 4p, 4d of Zn and 2s, 2p of O. RASSCF and RASPT2 calculations with (18,5+8+5)[2,2].

[e] Core orbitals not correlated at PT2 level: 1s, 2s, 2p, 3s, 3p of Zn (6,2,2,0).

**Table S12.** Vertical transition energies (eV) of ZnO with aug-cc-pVDZ basis set.

| State | Active space ($a_1,b_1,b_2,a_2$) | State-average ($A_1,B_1,B_2,A_2$) | CASSCF | CASPT2 NOIPEA (10 core)[b] | CASPT2 IPEA (10 core)[b] | SC-NEVPT2 (10 core)[b] | PC-NEVPT2 (10 core)[b] |
|---|---|---|---|---|---|---|---|
| $1^1\Pi$ | (6,3,3,1)[a] | (1,1,1,0) | 0.413 | **0.539** | **0.523** | **0.517** | **0.556** |
| $2^1\Sigma^+$ | (6,3,3,1)[a] | (2,0,0,0) | 3.594 | **3.689** | **3.767** | **3.789** | **3.720** |
| $1^1\Delta$ | (6,3,3,1)[a] | (2,0,0,1) | 4.181 | **4.186** | **4.365** | **4.386** | **4.399** |
| $1^1\Sigma^-$ | (6,3,3,1)[a] | (1,0,0,1) | 4.814 | **4.345** | **4.691** | **4.743** | **4.591** |
| $1^3\Pi$ | (6,3,3,1)[a] | (1,1,1,0) | 0.235 | **0.327** | **0.314** | **0.309** | **0.347** |
| $1^3\Sigma^+$ | (6,3,3,1)[a] | (2,0,0,0) | 1.373 | **1.538** | **1.590** | **1.575** | **1.578** |

[a] Using a reference (18e,13o) active space including 4s, 3d, 4p of Zn and 2s, 2p of O.

[b] Core orbitals not correlated at PT2 level: 1s, 2s, 2p, 3s, 3p of Zn (6,2,2,0).

**Table S13.** Vertical transition energies (eV) of ZnS with aug-cc-pVTZ basis set.

| State | Active space ($a_1,b_1,b_2,a_2$) | State-average ($A_1,B_1,B_2,A_2$) | CASSCF | CASPT2 NOIPEA (14 core)[b] | CASPT2 IPEA (14 core)[b] | SC-NEVPT2 (14 core)[b] | PC-NEVPT2 (14 core)[b] |
|---|---|---|---|---|---|---|---|
| $1^1\Pi$ | (5,3,3,0)[a] | (1,1,1,0) | 0.628 | **0.720** | **0.774** | **0.714** | **0.724** |
| $2^1\Sigma^+$ | (5,3,3,0)[a] | (2,0,0,0) | 3.852 | **3.856** | **3.978** | **3.973** | **3.915** |
| $1^1\Delta$ | (5,3,3,0)[a] | (2,0,0,1) | 4.053 | **4.046** | **4.231** | **4.209** | **4.216** |
| $1^1\Sigma^-$ | (5,3,3,0)[a] | (1,0,0,1) | 4.303 | **4.079** | **4.335** | **4.302** | **4.258** |
| $1^3\Pi$ | (5,3,3,0)[a] | (1,1,1,0) | 0.442 | **0.521** | **0.573** | **0.515** | **0.524** |
| $1^3\Sigma^+$ | (5,3,3,0)[a] | (2,0,0,0) | 2.040 | **2.249** | **2.314** | **2.314** | **2.306** |

[a] Using a reference (8e,11o) active space including 4s, 4p of Zn and 3s, 3p, $3d_{z^2}$, $3d_{xz}$, $3d_{yz}$ of S.

[b] Core orbitals not correlated at PT2 level: 1s, 2s, 2p, 3s, 3p of Zn and 1s, 2s, 2p of S (8,3,3,0).

**Table S14.** Vertical transition energies (eV) of ZnS with aug-cc-pVDZ basis set.

| State | Active space ($a_1,b_1,b_2,a_2$) | State-average ($A_1,B_1,B_2,A_2$) | CASSCF | CASPT2 NOIPEA (14 core)[b] | CASPT2 IPEA (14 core)[b] | SC-NEVPT2 (14 core)[b] | PC-NEVPT2 (14 core)[b] |
|---|---|---|---|---|---|---|---|
| $1^1\Pi$ | (5,3,3,0)[a] | (1,1,1,0) | 0.597 | **0.694** | **0.735** | **0.692** | **0.701** |
| $2^1\Sigma^+$ | (5,3,3,0)[a] | (2,0,0,0) | 3.853 | **3.865** | **3.974** | **3.968** | **3.911** |
| $1^1\Delta$ | (5,3,3,0)[a] | (2,0,0,1) | 4.042 | **4.042** | **4.198** | **4.185** | **4.191** |
| $1^1\Sigma^-$ | (5,3,3,0)[a] | (1,0,0,1) | 4.281 | **4.097** | **4.315** | **4.292** | **4.252** |
| $1^3\Pi$ | (5,3,3,0)[a] | (1,1,1,0) | 0.411 | **0.489** | **0.528** | **0.487** | **0.496** |
| $1^3\Sigma^+$ | (5,3,3,0)[a] | (2,0,0,0) | 2.069 | **2.256** | **2.311** | **2.312** | **2.304** |

[a] Using a reference (8e,11o) active space including 4s, 4p of Zn and 3s, 3p, $3d_{z^2}$, $3d_{xz}$, $3d_{yz}$ of S.

[b] Core orbitals not correlated at PT2 level: 1s, 2s, 2p, 3s, 3p of Zn and 1s, 2s, 2p of S (8,3,3,0).

## D. ScO and ScS

**Table S15.** Vertical transition energies (eV) of ScO with aug-cc-pVTZ basis set.

| State | Active space ($a_1,b_1,b_2,a_2$) | State-average ($A_1,B_1,B_2,A_2$) | CASSCF | CASPT2 NOIPEA (10 core)[c] | CASPT2 IPEA (10 core)[c] | CASPT2 NOIPEA (6 core)[d] | CASPT2 IPEA (6 core)[d] | SC-NEVPT2 (10 core)[c] | PC-NEVPT2 (10 core)[c] | SC-NEVPT2 (6 core)[d] | PC-NEVPT2 (6 core)[d] |
|---|---|---|---|---|---|---|---|---|---|---|---|
| $^2\Delta$ | (6,3,3,1)[a] | (2,0,0,1) | 1.855 | **1.812** | **1.794** | **1.678** | **1.684** | **1.773** | **1.797** | | |
| $^2\Pi$ | (6,3,3,1)[a] | (1,1,1,0) | 2.074 | **2.029** | **2.037** | **2.049** | **2.059** | **2.049** | **2.040** | | |
| $^2\Sigma^+$ | (7,3,3,1)[b] | (2,0,0,0) | 2.688 | **2.550** | **2.569** | **2.536** | **2.559** | **2.614** | **2.591** | **2.609** | **2.583** |
| $^2\Pi$ | (6,3,3,1)[a] | (1,2,2,0) | 3.349 | **3.655** | **3.632** | **3.601** | **3.583** | **3.527** | **3.502** | | |

[a] Using a reference (9e,13o) active space including 4s, 3d, 4p of Sc and 2s, 2p of O.

[b] Using a reference (9e,14o) active space including 4s, 3d, 4p, $4d_{z^2}$ of Sc and 2s, 2p of O.

[c] Core orbitals not correlated at PT2 level: 1s, 2s, 2p, 3s, 3p of Sc and 1s of O (6,2,2,0).

[d] Core orbitals not correlated at PT2 level: 1s, 2s, 2p of Sc and 1s of O (4,1,1,0).

**Table S16.** Vertical transition energies (eV) of ScO with aug-cc-pVDZ basis set.

| State | Active space ($a_1,b_1,b_2,a_2$) | State-average ($A_1,B_1,B_2,A_2$) | CASSCF | CASPT2 NOIPEA (10 core)[c] | CASPT2 IPEA (10 core)[c] | SC-NEVPT2 (10 core)[c] | PC-NEVPT2 (10 core)[c] |
|---|---|---|---|---|---|---|---|
| $^2\Delta$ | (6,3,3,1)[a] | (2,0,0,1) | 1.857 | **1.842** | **1.824** | **1.805** | **1.829** |
| $^2\Pi$ | (6,3,3,1)[a] | (1,1,1,0) | 2.067 | **2.024** | **2.032** | **2.044** | **2.036** |
| $^2\Sigma^+$ | (7,3,3,1)[b] | (2,0,0,0) | 2.678 | **2.557** | **2.575** | **2.616** | **2.594** |
| $^2\Pi$ | (6,3,3,1)[a] | (1,2,2,0) | 3.382 | **3.618** | **3.590** | **3.507** | **3.489** |

[a] Using a reference (9e,13o) active space including 4s, 3d, 4p of Sc and 2s, 2p of O.

[b] Using a reference (9e,14o) active space including 4s, 3d, 4p, $4d_{z^2}$ of Sc and 2s, 2p of O.

[c] Core orbitals not correlated at PT2 level: 1s, 2s, 2p, 3s, 3p of Sc and 1s of O (6,2,2,0).

**Table S17.** Vertical transition energies (eV) of ScS with aug-cc-pVTZ basis set.

| State | Active space ($a_1$,$b_1$,$b_2$,$a_2$) | State-average ($A_1$,$B_1$,$B_2$,$A_2$) | CASSCF | CASPT2 NOIPEA (14 core)[c] | CASPT2 IPEA (14 core)[c] | SC-NEVPT2 (14 core)[c] | PC-NEVPT2 (14 core)[c] |
|---|---|---|---|---|---|---|---|
| $^2\Delta$ | (5,2,2,1)[a] | (2,0,0,1) | 1.059 | **0.977** | **0.935** | | |
| | (6,3,3,2)[b] | (2,0,0,1) | 0.821 | **1.009** | **0.936** | **0.911** | **0.934** |
| $^2\Pi$ | (5,2,2,1)[a] | (1,1,1,0) | 2.032 | **1.627** | **1.739** | **1.736** | **1.608** |
| | (6,3,3,2)[b] | (1,1,1,0) | 1.512 | **1.498** | **1.476** | **1.485** | **1.434** |
| $^2\Sigma^+$ | (5,2,2,1)[a] | (2,0,0,0) | 1.680 | **1.518** | **1.566** | **1.523** | **1.566** |
| | (6,3,3,2)[b] | (2,0,0,0) | 1.768 | **1.587** | **1.634** | **1.633** | **1.574** |
| $^2\Pi$ | (5,2,2,1)[a] | (1,2,2,0) | 2.583 | **2.299** | **2.368** | | |
| | (6,3,3,2)[b] | (1,2,2,0) | 2.229 | **2.280** | **2.215** | **2.362** | **2.338** |

[a] Using a reference (9e,10o) active space including 4s, 3d of Sc and 3s, 3p of S.

[b] Using a reference (9e,14o) active space including 4s, 3d of Sc and 3s, 3p, four 3d of S.

[c] Core orbitals not correlated at PT2 level: 1s, 2s, 2p, 3s, 3p of Sc and 1s, 2s, 2p of S (8,3,3,0).

**Table S18.** Vertical transition energies (eV) of ScS with aug-cc-pVDZ basis set.

| State | Active space ($a_1$,$b_1$,$b_2$,$a_2$) | State-average ($A_1$,$B_1$,$B_2$,$A_2$) | CASSCF | CASPT2 NOIPEA (14 core)[b] | CASPT2 IPEA (14 core)[b] | SC-NEVPT2 (14 core)[b] | PC-NEVPT2 (14 core)[b] |
|---|---|---|---|---|---|---|---|
| $^2\Delta$ | (6,3,3,2)[a] | (2,0,0,1) | 0.851 | **1.050** | **0.981** | **0.954** | **0.974** |
| $^2\Pi$ | (6,3,3,2)[a] | (1,1,1,0) | 1.475 | **1.517** | **1.495** | **1.498** | **1.466** |
| $^2\Sigma^+$ | (6,3,3,2)[a] | (2,0,0,0) | 1.730 | **1.600** | **1.637** | **1.641** | **1.590** |
| $^2\Pi$ | (6,3,3,2)[a] | (1,2,2,0) | 2.022 | **2.149** | **2.134** | **2.153** | **2.140** |

[a] Using a reference (9e,14o) active space including 4s, 3d of Sc and 3s, 3p, four 3d of S.

[b] Core orbitals not correlated at PT2 level: 1s, 2s, 2p, 3s, 3p of Sc and 1s, 2s, 2p of S (8,3,3,0).

## E. TiN and ZnH

**Table S19.** Vertical transition energies (eV) of TiN with aug-cc-pVTZ basis set.

| State | Active space ($a_1,b_1,b_2,a_2$) | State-average ($A_1,B_1,B_2,A_2$) | CASSCF | CASPT2 NOIPEA (10 core)[b] | CASPT2 IPEA (10 core)[b] | SC-NEVPT2 (10 core)[b] | PC-NEVPT2 (10 core)[b] |
|---|---|---|---|---|---|---|---|
| $^2\Delta$ | (6,3,3,1)[a] | (2,0,0,1) | 1.038 | **0.855** | **0.840** | **0.884** | **0.874** |
| $^2\Pi$ | (6,3,3,1)[a] | (1,1,1,0) | 2.073 | **2.013** | **2.027** | **2.039** | **2.014** |
| $^2\Delta$ | (6,3,3,1)[a] | (3,0,0,2) | 2.181 | **2.118** | **2.227** | **2.242** | **2.222** |

[a] Using a reference (9e,13o) active space including 4s, 3d, 4p of Ti and 2s, 2p of N.
[b] Core orbitals not correlated at PT2 level: 1s, 2s, 2p, 3s, 3p of Ti and 1s of N (6,2,2,0).

**Table S20.** Vertical transition energies (eV) of TiN with aug-cc-pVDZ basis set.

| State | Active space ($a_1,b_1,b_2,a_2$) | State-average ($A_1,B_1,B_2,A_2$) | CASSCF | CASPT2 NOIPEA (10 core)[b] | CASPT2 IPEA (10 core)[b] | SC-NEVPT2 (10 core)[b] | PC-NEVPT2 (10 core)[b] |
|---|---|---|---|---|---|---|---|
| $^2\Delta$ | (6,3,3,1)[a] | (2,0,0,1) | 1.035 | **0.897** | **0.884** | **0.925** | **0.916** |
| $^2\Pi$ | (6,3,3,1)[a] | (1,1,1,0) | 2.074 | **2.031** | **2.045** | **2.054** | **2.030** |
| $^2\Delta$ | (6,3,3,1)[a] | (3,0,0,2) | 2.238 | **2.137** | **2.241** | **2.261** | **2.242** |

[a] Using a reference (9e,13o) active space including 4s, 3d, 4p of Ti and 2s, 2p of N.
[b] Core orbitals not correlated at PT2 level: 1s, 2s, 2p, 3s, 3p of Ti and 1s of N (6,2,2,0).

**Table S21.** Vertical transition energies (eV) of ZnH with aug-cc-pVTZ basis set.

| State | Active space ($a_1$,$b_1$,$b_2$,$a_2$) | State-average ($A_1$,$B_1$,$B_2$,$A_2$) | CASSCF | CASPT2 NOIPEA (9 core)[m] | CASPT2 IPEA (9 core)[m] | CASPT2 NOIPEA (5 core)[o] | CASPT2 IPEA (5 core)[o] | SC-NEVPT2 (9 core)[m] | PC-NEVPT2 (9 core)[m] |
|---|---|---|---|---|---|---|---|---|---|
| $1^2\Pi$ | (3,1,1,0)[a] | (1,1,1,0) | 2.657 | **2.799** | **2.818** | **2.800** | **2.819** | – | – |
| | (5,2,2,1)[b] | (1,1,1,0) | 2.682 | **2.830** | **2.851** | **2.833** | **2.853** | – | – |
| | (7,3,3,2)[c] | (1,1,1,0) | 2.713 | **2.838** | **2.862** | – | – | – | – |
| $2^2\Sigma^+$ | (3,1,1,0)[a] | (2,0,0,0) | 4.334 | **4.409** | **4.485** | **4.403** | **4.481** | **4.484** | **4.468** |
| | (5,2,2,1)[b] | (2,0,0,0) | 4.411 | **4.466** | **4.539** | **4.465** | **4.541** | **4.558** | **4.519** |
| | (7,3,3,2)[c] | (2,0,0,0) | 4.459 | **4.397** | **4.510** | – | – | – | – |
| $3^2\Sigma^+$ | (4,1,1,0)[d] | (3,0,0,0) | 4.733 | **5.056** | **5.040** | **5.038** | **5.022** | **5.028** | **5.021** |
| | (6,2,2,1)[e] | (3,0,0,0) | 4.765 | **5.091** | **5.093** | **5.082** | **5.083** | **5.067** | **5.041** |
| | (8,3,3,2)[f] | (3,0,0,0) | 4.839 | **5.089** | **5.097** | – | – | – | – |
| $4^2\Sigma^+$ | (5,1,1,0)[g] | (4,0,0,0) | 5.284 | **5.527** | **5.558** | **5.513** | **5.545** | **5.550** | **5.527** |
| | (7,2,2,1)[h] | (4,0,0,0) | 5.441 | **5.315** | **5.524** | – | – | – | – |
| | (9,3,3,2)[i] | (4,0,0,0) | 5.372 | **5.548**[n] | **5.598**[n] | – | – | – | – |
| $2^2\Pi$ | (3,2,2,0)[j] | (1,2,2,0) | 5.564 | **6.064** | **6.045** | **6.052** | **6.033** | – | – |
| | (5,3,3,1)[k] | (1,2,2,0) | 5.596 | **6.118** | **6.100** | **6.114** | **6.095** | – | – |
| | (7,4,4,2)[l] | (1,2,2,0) | 5.648 | **6.135**[n] | **6.106**[n] | – | – | – | – |

[a] Using a reference (3e,5o) active space including 4s, 4p of Zn and 1s of H.
[b] Using a reference (13e,10o) active space including 4s, 3d, 4p of Zn and 1s of H.
[c] Using a reference (13e,15o) active space including 4s, 3d, 4p, 4d of Zn and 1s of H.
[d] Using a reference (3e,6o) active space including 4s, 4p, 5s of Zn and 1s of H.
[e] Using a reference (13e,11o) active space including 4s, 3d, 4p, 5s of Zn and 1s of H.
[f] Using a reference (13e,16o) active space including 4s, 3d, 4p, 4d, 5s of Zn and 1s of H.
[g] Using a reference (3e,7o) active space including 4s, 4p, 5s, $5p_z$ of Zn and 1s of H.
[h] Using a reference (13e,12o) active space including 4s, 3d, 4p, 5s, $5p_z$ of Zn and 1s of H. (4p replaced by 4d)
[i] Using a reference (13e,17o) active space including 4s, 3d, 4p, 4d, 5s, $5p_z$ of Zn and 1s of H.
[j] Using a reference (3e,7o) active space including 4s, 4p, $5p_x$, $5p_y$ of Zn and 1s of H.
[k] Using a reference (13e,12o) active space including 4s, 3d, 4p, $5p_x$, $5p_y$ of Zn and 1s of H.
[l] Using a reference (13e,17o) active space including 4s, 3d, 4p, 4d, $5p_x$, $5p_y$ of Zn and 1s of H.
[m] Core orbitals not correlated at PT2 level: 1s, 2s, 2p, 3s, 3p of Zn (5,2,2,0).
[n] Using density-fitting.
[o] Core orbitals not correlated at PT2 level: 1s, 2s, 2p of Zn (3,1,1,0).

**Table S22.** Vertical transition energies (eV) of ZnH with aug-cc-pVDZ basis set.

| State | Active space ($a_1$,$b_1$,$b_2$,$a_2$) | State-average ($A_1$,$B_1$,$B_2$,$A_2$) | CASSCF | CASPT2 NOIPEA (9 core)[e] | CASPT2 IPEA (9 core)[e] |
|---|---|---|---|---|---|
| $1^2\Pi$ | (7,3,3,2)[a] | (1,1,1,0) | 2.713 | **2.820** | **2.843** |
| $2^2\Sigma^+$ | (7,3,3,2)[a] | (2,0,0,0) | 4.459 | **4.374** | **4.483** |
| $3^2\Sigma^+$ | (8,3,3,2)[b] | (3,0,0,0) | 4.846 | **5.054** | **5.062** |
| $4^2\Sigma^+$ | (9,3,3,2)[c] | (4,0,0,0) | 5.386 | **5.537**[f] | **5.582**[f] |
| $2^2\Pi$ | (7,4,4,2)[d] | (1,2,2,0) | 5.653 | **6.090**[f] | **6.062**[f] |

[a] Using a reference (13e,15o) active space including 4s, 3d, 4p, 4d of Zn and 1s of H.

[b] Using a reference (13e,16o) active space including 4s, 3d, 4p, 4d, 5s of Zn and 1s of H.

[c] Using a reference (13e,17o) active space including 4s, 3d, 4p, 4d, 5s, $5p_z$ of Zn and 1s of H.

[d] Using a reference (13e,17o) active space including 4s, 3d, 4p, 4d, $5p_x$, $5p_y$ of Zn and 1s of H.

[e] Core orbitals not correlated at PT2 level: 1s, 2s, 2p, 3s, 3p of Zn (5,2,2,0).

[f] Using density-fitting.
